# Supplementary material for: A Graph-Based Neural Model for End-to-End Frame Semantic Parsing
Source: arXiv:2109.12319 source file (2021-09-25)
Supplement: Supplementary file 1 [file appendix.tex]

\documentclass[11pt,a4paper]{article}
\usepackage[hyperref]{emnlp2021}
\usepackage{times}
\usepackage{latexsym}
\usepackage{bm}
\usepackage{amsmath,amssymb}
\usepackage{graphicx}
\usepackage{multirow}
\usepackage{booktabs}
\usepackage{subfigure}
\usepackage{color}
\usepackage{CJK}

% This is not strictly necessary, and may be commented out,
% but it will improve the layout of the manuscript,
% and will typically save some space.
\usepackage{microtype}

%\aclfinalcopy % Uncomment this line for the final submission
 %  Enter the acl Paper ID here

%\setlength\titlebox{5cm}
% You can expand the titlebox if you need extra space
% to show all the authors. Please do not make the titlebox
% smaller than 5cm (the original size); we will check this
% in the camera-ready version and ask you to change it back.

%\newcommand{\zms}[1]{\textcolor{red}{zms: #1}}
%\newcommand{\zx}[1]{\textcolor{red}{zx: #1}}
%\hypersetup{draft}

\begin{document}
\begin{CJK}{UTF8}{gbsn}
\appendix

\section{Hyper-parameters}
\end{CJK}
\end{document}
